# Supplementary material for: Giant transverse magnetic fluctuations at the edge of re-entrant superconductivity in UTe$_{2}$
Source: arXiv:2506.08984 source file (2025-06-10)
Supplement: Supplementary file 1 [file SI.pdf]

# Supplementary information for "Giant transverse magnetic susceptibility at the edge of re-entrant superconductivity in $UTe_2$"

## I. CRYSTAL SYNTHESIS

Crystal was synthesized using the chemical vapor transport method, with iodine as the transport agent and a 5:9 starting ratio of U:Te. The sample was grown in a temperature gradient of 900/830°C for two weeks. Between measurements, the samples were stored in vacuum.

## II. CRYSTAL AXES & ALIGNMENT

Accurate measurements of the magnetotropic susceptibility $k = \partial^2 F/\partial\theta^2$ are sensitive to the alignment of the crystallographic axes with respect to the external magnetic field. In order to identify the crystallographic axes, we performed x-ray scattering using a commercial Laue detector from Photonic Science. Figure 1 shows the $a$- and $b$-axes of the orthorhombic structure of $UTe_2$.

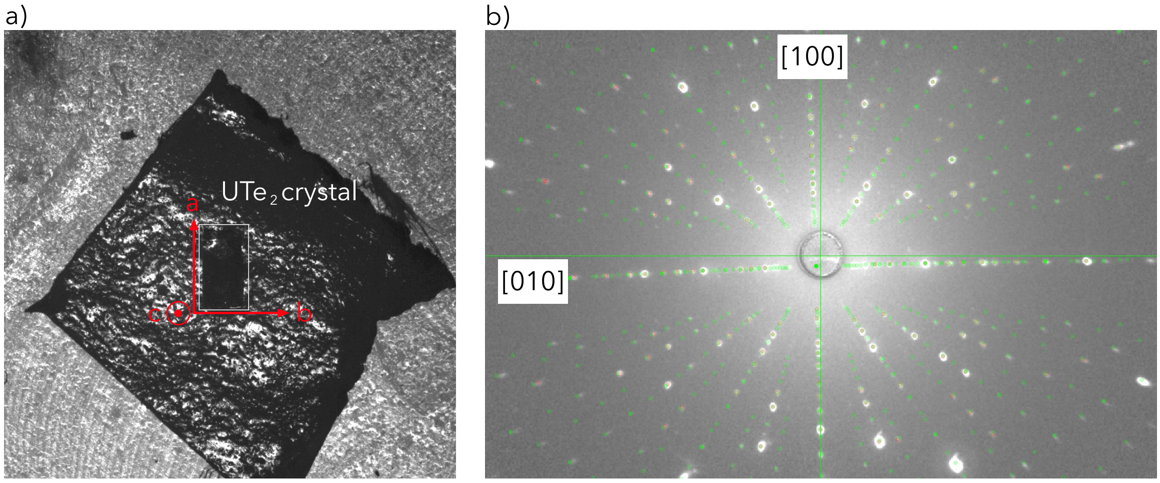


FIG. 1. **Laue diffraction on Sample #2** The crystal was mounted with the $c$-axis perpendicular to the surface of a scanning electron microscopy (SEM) stub. An example of the diffraction spectra showing the alignment of the $a$-axis and $b$-axis relative to the sample.

After identifying the $a$- and $b$-axis using the Laue, the axes were marked on the stub and were kept track of when cutting small pieces off for Sample #2 and Sample #3, and for cutting in the FIB chamber for sample #1.

## III. SAMPLE PREPARATION

In highly-anisotropic materials, magnetotropic signal sizes vary substantially with magnetic field orientation. In order to achieve an appropriate signal size in the magnetotropic measurements for magnetic field rotated throughout these highly-anisotropic planes (i.e. to avoid breaking the cantilever), we need to prepare small samples. In total, we prepared 3 samples from 2 different bulk pieces (separate single crystals from the same batch). Two samples were cut by hand, and for one sample (Sample #1 used in the main text) we used the Helios G4 xenon plasma focused-ion beam (FIB). Use of the FIB allowed for better sample alignment. The overall trends in the high-field results, from both the $ac$- and $bc$-plane measurement, are consistent between all three samples, with slight differences due to misalignment and the high sensitivity of $UTe_2$ to field angle. Sample information is summarized in Table I below.

TABLE I. Summary of the samples measured and their relevant parameters

| Sample | Bulk | Type | Volume [$\mu m^3$] | mol of U | $k$ for 1 Hz [J/mol] |
|---|---|---|---|---|---|
| 1 | A | FIB'ed | 72,914 | $1.36 \times 10^{-9}$ | 0.77 |
| 2 | B | Hand cut | 456,624 | $8.53 \times 10^{-9}$ | 0.54 |
| 3 | B | Hand cut | 568,620 | $1.06 \times 10^{-8}$ | 0.43 |

Once the crystal axes were identified with respect to the macroscopic crystal, the sample was mounted with the $b$-axis perpendicular to the surface of the sample holder and placed into the FIB chamber (Figure 2). Samples were cut from the bulk single crystal using small currents (4-15 nA) at 20 kV to minimize sample heating and surface damage.

After cutting and polishing the sides of the samples using the ion beam, the samples were left hanging from the bulk crystal by a $\sim 1 \times 1\ \mu\text{m}^2$ bridge. Under an optical microscope, Sample #1 was manually disconnected from the bulk piece using an eyelash and a kapton needle. Before transferring the sample to the silicon microcantilever for measurements, a small drop of Apiezon L grease was placed on the lever to ensure that magnetic torque on the sample during measurements does not displace it. After measurements, we check that the placement of the sample on the lever remained intact.

Sample #2 and Sample #3 were cut using a razor blade from a different bulk sample than Sample #1. Before cutting the crystal, we used Laue to confirm the crystal axes. We then painted each face a different color in order to correlate the crystal axes in the cut piece with those from the Laue results.

For both measurement planes, the $c$-axis of the sample was mounted perpendicular to the surface of the lever and the $a$- or $b$-axis was mounted parallel to the long axis of the lever, depending upon the plane of anisotropy to be measured ($ac$- or $bc$-plane). After measurements in the first plane, the sample was rotated under an optical microscope by hand by $\sim 90°$.

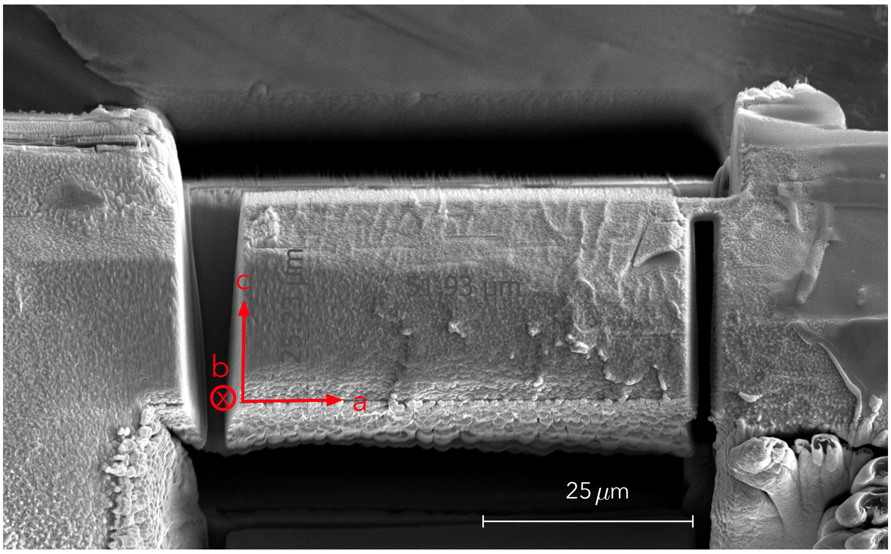


FIG. 2. **FIB'ed $UTe_2$ Sample #1** The dimensions are $\sim 52 \times 66 \times 25\ \mu\text{m}^3$.

## IV. MAGNETOTROPIC MEASUREMENTS

We used the Nanosensors Akiyama-probe – a commercial silicon microcantilever developed for atomic force microscopy [1, 2]. The lever is connected to a quartz tuning fork that electrically drives and detects the resonance frequency of the coupled (fork + lever) oscillators. By operating at the fundamental bending mode of the lever, which ranges from $\sim$ 35 to 40 kHz, we probe anisotropy in the plane of the principal axes that are in the plane of oscillation and field rotation [4].

The magnetotropic measurements were carried out at the National High Magnetic Field Laboratory (NHMFL) in Los Alamos National Laboratory, USA. The tuning fork with the cantilever attached was mounted onto a G10 substrate. The substrate is designed to ensure proper alignment and contact between the fork and the substrate. The G10 substrate is then attached to the stage of the rotator probe. The probe is then inserted into a vacuum-walled stainless steel fridge and the probe space is pumped down to $10^{-5}$ mbar. The fridge is inserted into a helium-4 cryostat. By introducing a small amount of exchange gas into the sample space, the sample reaches $T = 4$ K (note that atmospheric pressure in Los Alamos is substantially lower than at sea level and liquid helium is close to 4 K at these altitutes). In order to avoid the magnetic response of the superconductivity itself, a majority of our measurements were performed at 4 K. However, for a few measurements, we pumped on the bath of helium-4 to reach $T = 1.6$ K and measured below $T_c$ (Figure 3).

A frequency scan is performed once the measurement temperature is stable to identify the resonant frequency. We drive the cantilever at its resonance frequency before the field pulse and then, just before discharging the capacitor bank to the magnet, a trigger signal is sent to stop the cantilever drive and the cantilever oscillates freely. Throughout the magnetic field pulse, the magnetotropic susceptibility leads to shifts in the oscillation frequency, and the raw data is collected with a digitizer for post-processing. The magnetic field versus time has a full-width at half maximum of $\sim$10 ms. The total duration of the pulse, including its slow decay, is $\sim$100 ms. By the end of the pulse, the amplitude of the resonant frequency, which is also consistently monitored, decays to about 50% of its drive value. With a resonance frequency of roughly 40 kHz, a single lever oscillation cycle occurs in 25 $\mu$s. Several oscillations are analyzed over small time windows of 100-250 $\mu$s to find the resonance frequency, and the windows are stepped by 20 $\mu$s to generate

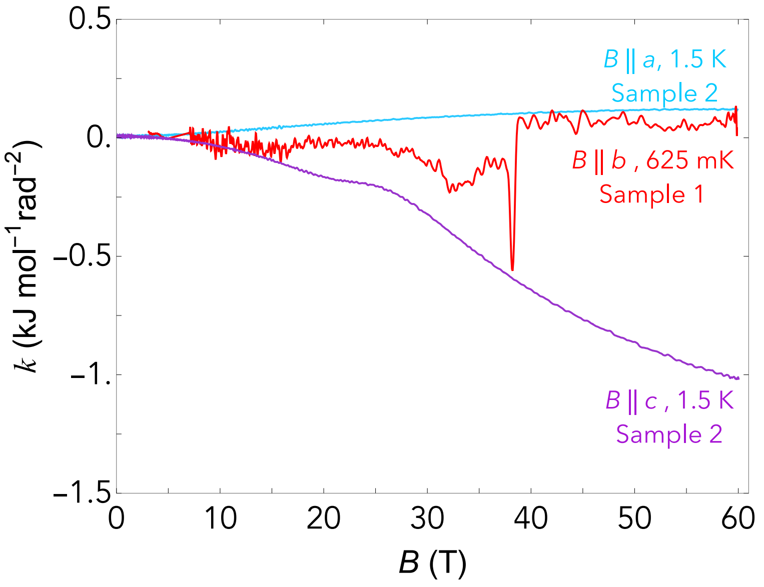


FIG. 3. **Magnetotropic measurements in the superconducting state** At temperatures below $T_c$ (1.85 K in our samples), the magnetotropic susceptibility versus magnetic field for the three crystallographic directions. On Sample #1, $k$ was measured for $B||b$ at $T$ = 625 mK. The large increase in noise is due to the reduction in vibration damping because the 4He bath is superfluid at these temperatures. The onset of the magnetotropic softening – small at this angle – is visible as a downturn near 25 T as a precursor to the metamagnetic transition near 35 T. The large magnetotropic softening near 20 T in Sample #2 at 1.5 K reproduces the main finding in the manuscript observed in the $bc$-plane for Sample #1. The blue curve shows $k$ for $B||a$, also for Sample #2, which exhibits an essentially flat response up to 60 T – again consistent with Figure 2c in the manuscript.

each data point. The zero-field frequency is always remeasured between measurements taken at new field angles (*i.e.* after rotating the sample).

### IV.1. Reproducibility

We performed high-field magnetotropic measurements on two different bulk crystals: Sample #1 was FIB'ed and Samples #2 and #3 were cut from a bulk piece using a razor blade. The data included in the main text was taken from Sample #1. We also acquired data in the $ac$- and $bc$-planes for Sample #2 and Sample #3. We find that the data taken across all samples is consistent; in particular, the large decrease in magnetotropic susceptibility, indicating a large increase in transverse susceptibility in the $bc$ plane, is consistent between samples.

Figure 3 shows the magnetotropic susceptibility taken at temperatures below $T_c$ for field aligned along each of the crystallographic directions in two different samples. The red curve shows data taken at the lowest temperature of 625 mK. The overall features observed in Figure 2 c&d at $T$ = 4 K in the manuscript are reproduced here in Figure 3. The key consistencies are: i) the overall magnitude of the signal for all field configurations (*i.e.* a small response for $B||a$ and $B||b$ up to 60 T) ii) the onset of softening near 20 T and the metamagnetic transition near 35 T for $B||b$, and iii) the large softening that onsets near 20 T for $B||c$. This also demonstrates that the transverse softening persists down to low temperatures.

Figure 4 demonstrates that the main findings observed in the magnetotropic susceptibility in Sample #1 (a FIB'ed sample) of the manuscript are reproduced here for two different samples. In particular, we find 1) a large softening observed at ∼20 T for a wide range of angles in both the $ac$- and $bc$-plane and 2) a critical endpoint to the line of first-order metamagnetic transitions in the $bc$-plane. In Sample #3, we observe that the softening onsets at a slightly lower field of ∼10 T compared to ∼20 T in Sample #1 in the manuscript. We also observe a large discontinuity in the middle of the field range over which the softening occurs for several angles near the $c$-axis, for measurements both in the $ac$- and $bc$-planes. This jump down followed by a peak in the magnetotropic susceptibility upon approaching 20 T is characteristic of a second-order phase transition, which was not observed in Sample #1. We attribute this difference to slight misalignments of the $bc$-plane on the lever for both samples; we believe in Sample #1, we precess around the phase transition observed in Sample #3. This is in agreement with the fact that the metamagnetic transition and the critical endpoint also occur at slightly different angles in both experiments. Alignment of our samples, which are only 100's of nanograms, is a technical challenge. As all features in $UTe_2$ are highly-anisotropic, one expects that slight misalignments may lead to variation in the positions of features observed with angle. Assuming ≈ 10° offsets, our data are consistent with that of Lewin et al. [3].

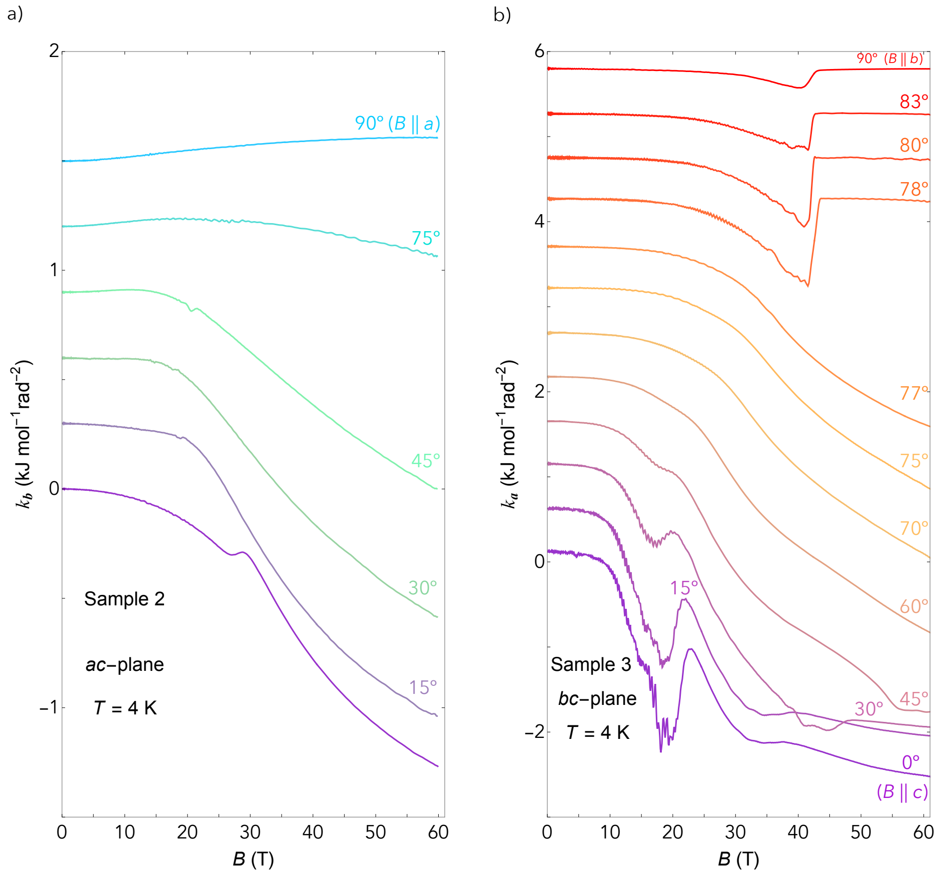


FIG. 4. **Magnetotropic susceptibility in the $ac$- and $bc$-planes** a) The $ac$-plane of Sample #2 was rotated with respect to field for several 60 T magnetic field pulses. A large decrease in the magnetotropic susceptibility is observed, similar in magnitude to that observed in Figure 2 of the main text. b) For rotation in the $bc$-plane, a large decrease in the magnetotropic susceptibility is again observed in a region consistent with the data shown in the main text. Between $\theta = 77^\circ$ and $\theta = 78^\circ$, the softening is cut off by the metamagnetic phase boundary that extends from $B||b$. The difference in $B^\star$ between this data and the data in the main text is due to a great degree of sample misalignment for this sample. However, the features as a function of angle are consistent with other studies if we assume an angle offset [3]. A large discontinuity indicating a possible second-order phase transition—possibly the $B^\star$ line from the second-order endpoint of the metamagnetic transition—is observed near 20 T in Sample #3.

## V. CALIBRATION

In order to convert the measured frequency into the correct magnetotropic susceptibility units (J/mol/rad$^2$), we use the linear response regime $M_i = \chi_{ij} H_j$. Here, the frequency shift, which is directly proportional to the magnetotropic susceptibility, follows a characteristic field- and angle-dependence $k = (\chi_i - \chi_j)\cos 2\theta B^2$, where $i, j$ describe the principal magnetic axes of the crystal in the plane of oscillation. Figure 5 shows the measured frequency shift vs $B$ after subtracting their respective zero-field frequencies. After subtraction, a quadratic fit to the low-field (from ~1-7 T) data gives the proportionality factor of the magnetic anisotropy.

A plot of the coefficient to the quadratic behavior in Figure 5a versus angle yields the anisotropy in the magnetic susceptibility, $\chi_i - \chi_j$ (Figure 5b). At $\theta = 0^\circ$, the amplitude is $\sim$ -0.47 Hz/T$^2$. The anisotropic susceptibility obtained through magnetic susceptibility measurements for field aligned along the $a$- and $c$-axes is $\chi_a - \chi_c = 0.36$ J/T$^2$/mol [5]. This can be equated with the amplitude of angle-dependent $k$ measurements

$$0.47 \left[\frac{\text{Hz}}{\text{T}^2}\right] \rightarrow 0.36 \left[\frac{\text{J}}{\text{T}^2\ \text{mol}}\right] \tag{1}$$

Therefore, the conversion factor applied to the magnetotropic measurements for Sample #1 is 1 Hz $\rightarrow$ 0.77 J/mol/rad$^2$.

Because the anisotropy in the $bc$-plane at low fields is so small, the same calibration factor was applied to the $bc$-plane data for unit conversion. This is valid because we use the same sample on the same cantilever, and thus the calibration factor—related to the bending stiffness of the cantilever—is the same.

The magnetotropic susceptibility divided by magnetic field can be represented in units of magnetization. Based on the volume of the sample, the unit cell volume, and the fact that each (conventional) unit cell has 4 uranium atoms, we estimate 1.36$\times$10$^{-9}$ moles of uranium in Sample #1. With $\mu_B = 9.2 \times 10^{-24}$ J/T, this allows for conversion of the frequency shift into units of $\mu_B$ per U:

$$1 \left[\frac{\text{Hz}}{\text{T}}\right] \rightarrow 0.14 \left[\frac{\mu_B}{\text{U}}\right]. \tag{2}$$

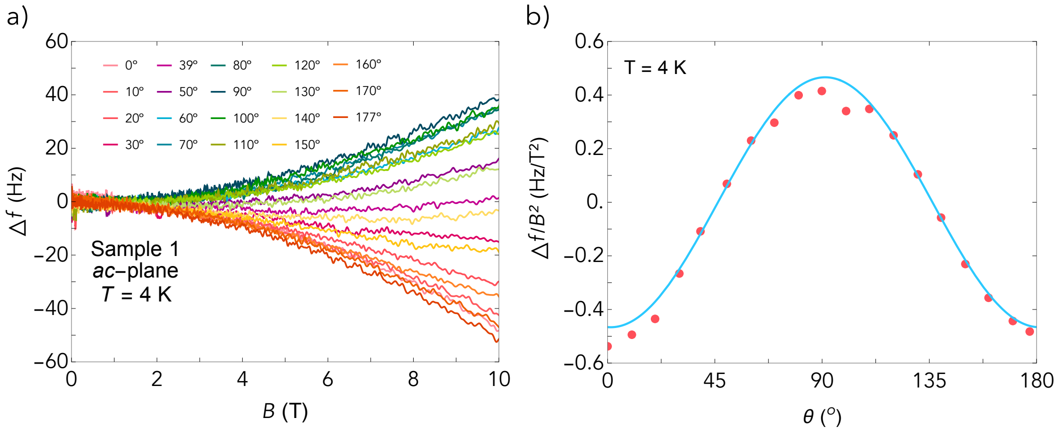


FIG. 5. **Magnetotropic susceptibility at low fields on Sample #1 in the** $ac$**-plane** a) At $T = 4$ K, the measured frequency shift after subtracting the zero-field frequency versus magnetic field up to 10 T at various field orientations. The frequency shift is proportional to the magnetotropic susceptibility, which has a quadratic field dependence at low fields due to a linear-in-field magnetization. b) The coefficient to the quadratic-in-field dependence of the magnetotropic susceptibility follows a cos$2\theta$ dependence and is proportional to the anisotropic magnetic susceptibility in the plane of vibration $(\chi_i - \chi_j)$.


[1] Terunobu Akiyama, Nicolaas F. de Rooij, Urs Staufer, Manfred Detterbeck, Dominik Braendlin, Simon Waldmeier, and Martin Scheidiger. Implementation and characterization of a quartz tuning fork based probe consisted of discrete resonators for dynamic mode atomic force microscopy. *Review of Scientific Instruments*, 81(6):063706, 2010. ISSN 0034-6748. doi: 10.1063/1.3455219.

[2] Wilton J M Kort-Kamp, Ryan A Murdick, Han Htoon, and Andrew C Jones. Utilization of coupled eigenmodes in Akiyama atomic force microscopy probes for bimodal multifrequency sensing. *Nanotechnology*, 33(45):455501, 2022. ISSN 0957-4484. doi:10.1088/1361-6528/ac8232.

[3] Sylvia K Lewin, Peter Czajka, Corey E Frank, Gicela Saucedo Salas, Hyeok Yoon, Yun Suk Eo, Johnpierre Paglione, Andriy H Nevidomskyy, John Singleton, and Nicholas P Butch. High-Field Superconducting Halo in UTe$_2$$. *arXiv*, 2024. doi:10.48550/arxiv.2402.18564.

[4] K. A. Modic, Maja D. Bachmann, B. J. Ramshaw, F. Arnold, K. R. Shirer, Amelia Estry, J. B. Betts, Nirmal J. Ghimire, E. D. Bauer, Marcus Schmidt, Michael Baenitz, E. Svanidze, Ross D. McDonald, Arkady Shekhter, and Philip J.W. Moll. Resonant torsion magnetometry in anisotropic quantum materials. *Nature Communications 2018 9:1*, 9:1–8, 9 2018. doi: 10.1038/s41467-018-06412-w. URL https://www.nature.com/articles/s41467-018-06412-w.

[5] Priscila F. S. Rosa, Ashley Weiland, Shannon S. Fender, Brian L. Scott, Filip Ronning, Joe D. Thompson, Eric D. Bauer, and Sean M. Thomas. Single thermodynamic transition at 2 K in superconducting UTe2 single crystals. *Communications Materials*, 3(1):33, 2022. doi:10.1038/s43246-022-00254-2.
